# Supplementary material for: Phonon-induced enhancement of photon entanglement in quantum dot-cavity systems
Source: arXiv:1902.04933 ancillary file (2019-09-25)
Supplement: Supplementary file 1 [file Supplement.pdf]

# Supplement: Phonon-induced enhancement of photon entanglement in quantum dot-cavity systems

T. Seidelmann,[1] F. Ungar,[1] A. M. Barth,[1] A. Vagov,[1,2] V. M. Axt,[1] M. Cygorek,[3] and T. Kuhn[4]

[1] *Universität Bayreuth, Lehrstuhl für Theoretische Physik III, Universitätsstraße 30, 95447 Bayreuth, Germany*
[2] *ITMO University, St. Petersburg, 197101, Russia*
[3] *Department of Physics, University of Ottawa, Ottawa, Ontario, Canada K1N 6N5*
[4] *Institut für Festkörpertheorie, Universität Münster, 48149 Münster, Germany*

## CONCURRENCE OF SIMULTANEOUSLY EMITTED PHOTONS

The concurrence is a widely used measure for the entanglement of a bipartite system. It has a one-to-one correspondence to the entanglement of formation [1] which represents the amount of pure-state entanglement that is at least present in a mixed state described by a given density matrix. Even though the entanglement of formation is more intuitive, the concurrence is usually preferred since it can be extracted directly from the values of the reduced density matrix of the bipartite system for which the entanglement is to be measured [2].

It is worthwhile to note that the photons emitted from the biexciton-exciton cascade can be subdivided in different ways into bipartite subsystems [3]. The associated concurrences are not necessarily equivalent since they may exhibit opposite trends when varying parameters such as, e.g., the cavity losses [3]. Widely used is the concurrence of all photon pairs that are detected in coincidence measurements without discriminating between the detection times of the two photons [3–7]. This choice results in a high signal yield but measurements [8, 9] as well as theoretical considerations [3, 10] indicate that significantly higher degrees of entanglement can be reached by selecting simultaneously emitted photon pairs. For this reason the concurrence of simultaneously emitted pairs is preferred in the present study. The more general expression given in Ref. [2] reduces in our case to

$$C = 2\,|\bar{\rho}^N_{HV}|, \tag{S1}$$

where the normalized two-photon coherence

$$\bar{\rho}^N_{HV} = \frac{\bar{\rho}_{HV}}{\bar{\rho}_{HH} + \bar{\rho}_{VV}} \tag{S2}$$

is calculated from the time-averaged elements of the reduced density matrix

$$\bar{\rho}_{mn} = \frac{1}{T_{\rm av}} \int_0^{T_{\rm av}} \langle mm|\hat{\rho}(t)|nn\rangle \, {\rm d}t. \tag{S3}$$

Here, $|HH\rangle := |G,2,0\rangle$ ($|VV\rangle := |G,0,2\rangle$) denotes the state with two horizontally (vertically) polarized photons. The averaging is performed until the time $T_{\rm av}$ is reached where the initially prepared biexciton has fully decayed and the system has reached its ground state without any photons inside the cavity.

In experiments, the two-photon density matrix, from which the concurrence can be derived, is usually reconstructed using quantum state tomography, a technique based on polarization-dependent photon coincidence measurements [11]. This technique gives access to information about the polarization degree of freedom and the delay time between the two detection events. The concurrence of simultaneously emitted photon pairs can be obtained from the reconstructed density matrix elements in the limit where the delay time approaches zero. Typically, in the corresponding experiments, data points are recorded over extended delay time intervals. Here, the limit of zero delay time can be approached by using time-windowing techniques where signals over different delay time windows are recorded and then the data is extrapolated towards zero delay time [8, 9].

## RENORMALIZATION OF THE QUANTUM DOT-CAVITY COUPLING

In the main text we argue that the shift of the minimum in the concurrence plotted versus the dot-cavity coupling $g$ is caused by the phonon-induced renormalization of $g$. This renormalization occurs already in a two-level system

where it is much simpler to analyze than in the five-level system considered in the present manuscript. For vanishing biexciton binding energy and the usually not very large fine-structure splitting, the transitions from the biexciton to the exciton states and from the exciton states to the ground state are similar and their phonon-induced renormalization can be expected to be close to the case of resonant coupling. Therefore, we followed Ref. [12] in order to obtain a simple estimate for the renormalization, i.e., we have performed path-integral calculations for a resonantly driven two-level system with the same dot and phonon parameters as used in the main text but for $\kappa = 0$. For driving with constant amplitude the exciton occupation is well fitted by the expression:

$$\rho_X = \frac{1}{2}\left[1 - e^{-\Gamma t}\cos(\omega t)\right], \tag{S4}$$

where $\Gamma = \Gamma(g,T)$ and $\omega = \omega(g,T)$ are used as fitting parameters. As explained in detail in Ref. [12], the renormalized dot-cavity coupling is related to $\Gamma$ and $\omega$ by:

$$\tilde{g}(g,T) = [\Gamma^2(g,T) + \omega^2(g,T)]/(4g) \tag{S5}$$

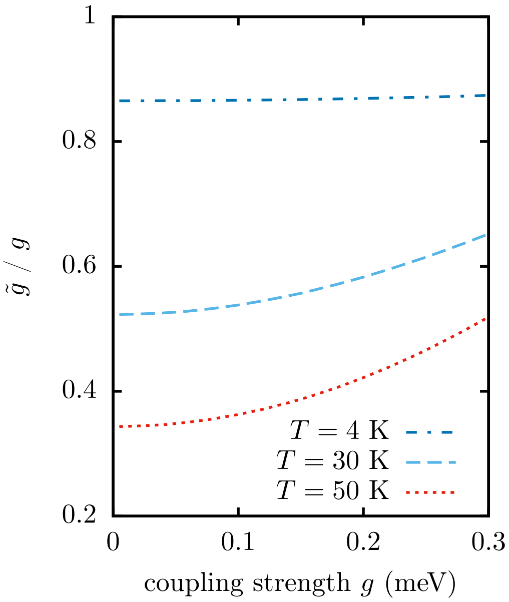


FIG. S1. Renormalized dot-cavity coupling $\tilde{g}(g,T)/g$ as a function of the original coupling $g$ for different temperatures.

Figure S1 displays the resulting renormalized dot-cavity coupling as a function of the original coupling for different temperatures. Clearly, for not too high values of $g$ (which constitutes the typical situation) the phonon renormalization leads to a reduction of the effective coupling. Thus, in order to achieve the same effect with the renormalized $g$ as without renormalization one needs to increase the bare value of $g$, which explains why the minimum in Fig. 1(c) in the main text is shifted to higher $g$ values.

## PHONON-INDUCED ENTANGLEMENT FOR DEGENERATE EXCITONS AND FINITE CAVITY MODE SPLITTING

In this section we present numerical simulations of the concurrence for the situation sketched in Fig. S2(a), i.e., a system with vanishing biexciton binding energy, degenerate excitons and cavity modes with a finite splitting given by $\delta^c = \hbar(\omega_H^c - \omega_V^c)$. Since the excitons are degenerate, which-path information is introduced in this configuration only by the cavity mode splitting.

The concurrence is again a non-monotonic function of $g$ already in the phonon-free case [purple curve in Fig. S2(c)]. However, the situation here is more involved than in Fig. 1(c) in the main text, since instead of a single minimum we now have two well pronounced minima. Accounting for phonons, we observe also in this configuration a clear shift of the curves toward higher $g$ values with rising temperature accompanied by an overall lowering of the curves. As in

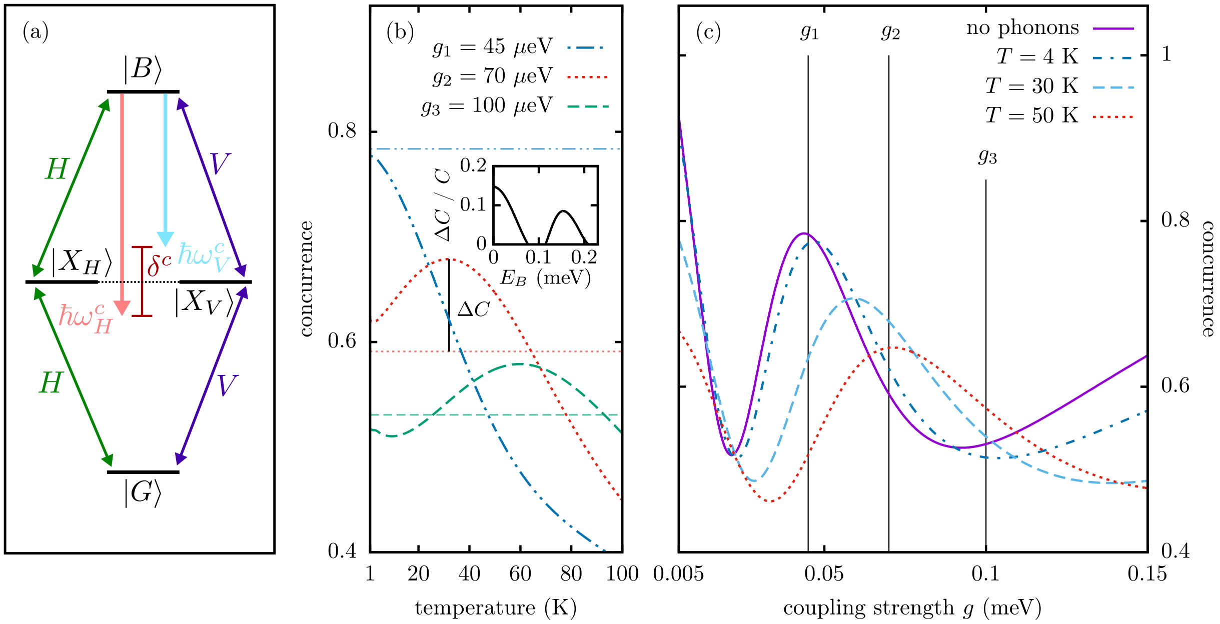


FIG. S2. (a) Sketch of the level scheme of a QD-cavity system with finite cavity mode splitting, zero biexciton binding energy, and degenerate excitons. (b) Concurrence as a function of the temperature for three selected values of the QD-cavity coupling. The corresponding values obtained without phonons are drawn as straight (faded) lines with the same linetype. The inset shows the difference $\Delta C$ between the maximum concurrence value at a finite temperature and the corresponding phonon-free value (only positive values are shown) normalized by the latter as a function of the biexciton binding energy $E_B$ for $g_2 = 70$ μeV. In the case of a finite $E_B$, the cavity modes are adjusted such that their mean energy coincides with the degenerate exciton energy $\hbar\omega_X$: $\hbar\omega^c_{H/V} = \hbar\omega_X \pm \delta^c/2$. (c) Concurrence as a function of the QD-cavity coupling for three temperatures together with the phonon-free result. The values of the QD-cavity coupling used in (b) are marked in (c) by vertical lines. Parameters: $\delta^c = 0.07$ meV, $\kappa = 0.05\,\mathrm{ps}^{-1}$. All other parameters are the same as in Fig. 1 in the main text.

Fig. 1(c) in the main text also here the shift caused by the renormalization is the dominant phonon-induced effect and consequently the temperature dependence of the concurrence depends crucially on the chosen value of $g$ [cf. Fig. S2(b)]. For example, for $g = 45\,\mu$eV we find the usually encountered monotonic decrease with rising temperature. In contrast, for $g = 70\,\mu$eV and $g = 100\,\mu$eV the concurrence exhibits different non-monotonic temperature dependences. In both cases extended ranges for $g$ are found where the concurrence reaches values above the corresponding phonon-free level. This demonstrates that the phenomenon of phonon-induced entanglement as described in the main text can also be observed in a configuration where the cavity modes are split while the excitons are degenerate and the biexciton binding is weak. Again, similar to the configuration discussed in the main text, this effect occurs for a finite range of biexciton binding energies [cf. inset panel (b)]. Here, the effect can be observed even when the binding energy is a few times the value of the splitting $\delta^c$.

## DEPENDENCE ON THE BIEXCITON BINDING ENERGY

The effect of phonon-induced enhancement of photon entanglement does not only occur in the singular case of a vanishing biexciton binding energy but rather for a finite range of binding energies depending on the respective splitting. It is worthwhile to note that apart from the natural occurrence of QDs with small biexciton binding energies, the biexciton binding energy can also be tuned into this regime, e.g., by the application of an electrical field [13] or a biaxial strain [14, 15], or both combined [16]. In the main text, the case of a vanishing and a finite (large) $E_B$ value are discussed in detail and presented in Figs. 1 and 2 for a quantum dot-cavity system with finite fine-structure splitting and two photon resonant cavity modes. While in the first case phonon-induced enhancement can be observed this effect does not occur in the latter one. A continuous transition between these two types of behavior is expected.

Figure S3 shows the dependence on the biexciton binding energy $E_B$ of the difference $\Delta C$ between the maximum concurrence value at a finite temperature and the corresponding phonon-free value normalized by the latter one. Figure S3(a) displays results for the situation considered in the main text where the cavity modes are degenerate

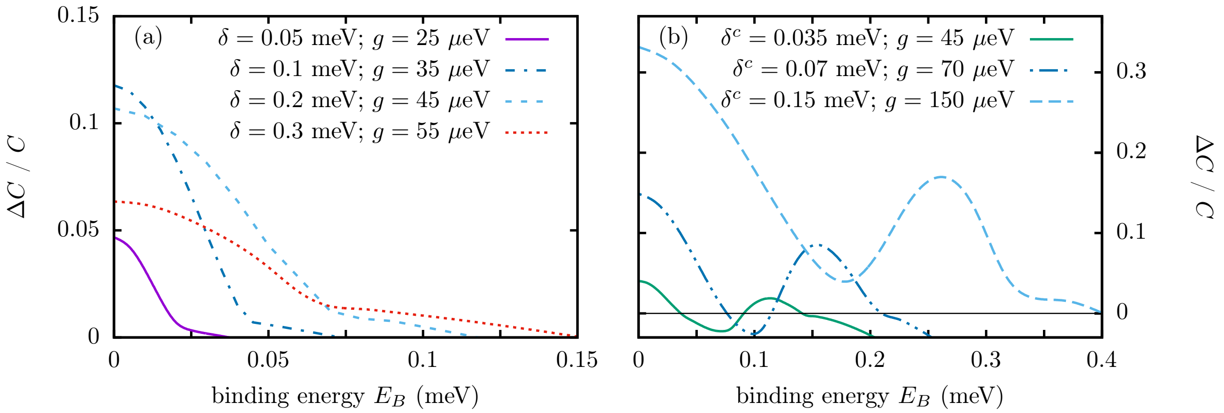


FIG. S3. Difference $\Delta C$ between the maximum concurrence value at a finite temperature and the corresponding phonon-free value normalized by the latter as a function of the biexciton binding energy $E_B$. (a) Results for a QD-cavity system with two-photon resonant cavity modes and cavity loss rate $\kappa = 0.025$ ps$^{-1}$ for four different combinations of finite fine-structure splittings $\delta$ and light-matter coupling strengths $g$. Corresponding level schemes can be found in the main text in Figs. 1 and 2. (b) Results for a QD-cavity system with degenerate excitons and cavity loss rate $\kappa = 0.05$ ps$^{-1}$ for three different combinations of finite cavity mode splittings $\delta^c$ and light-matter coupling strengths $g$. The corresponding level scheme for a vanishing $E_B$ can be found in Fig. S2. In the case of a finite binding energy, the cavity modes are adjusted such that their mean energy coincides with the degenerate exciton energy $\hbar\omega_X$: $\hbar\omega^c_{H/V} = \hbar\omega_X \pm \delta^c/2$.

and the excitons exhibit a finite fine-structure splitting $\delta$, while the curves in Figure S3(b) are obtained for the case described in the previous section where the excitons are degenerate and the cavity modes are split. Different combinations of exciton (cavity mode) splittings $\delta$ ($\delta^c$) and coupling strengths $g$ are considered. Indeed, in both QD-cavity configurations discussed in the main text and the supplement, which exhibit phonon-induced enhancement of photon entanglement, this effect occurs for a finite range of binding energies. For both configurations this range is roughly proportional to the respective splitting $\delta$ or $\delta^c$. In the case of a QD-system with a finite fine-structure splitting $\delta$ and two-photon resonant cavity modes, the effect can be seen until the binding energy reaches approximately half the value of the splitting $\delta$ [cf. Fig. S3(a)].

For the second QD-cavity configuration [Fig. S3(b), degenerate exciton energies, finite cavity mode splitting $\delta^c$] the situation is more involved since $\Delta C$ turns out to depend non-monotonically on $E_B$. Nevertheless, also here a finite range of binding energies exists where phonon-induced enhancement of photon entanglement can be found. Again this range is roughly proportional to the splitting $\delta^c$. For some combinations of $g$ and $\delta^c$, the value of $\Delta C$ first drops below zero and then phonon-induced entanglement enhancement is recovered at higher values of $E_B$, while for other combinations the minimum of $\Delta C$ as a function of $E_B$ has a positive value. In all cases, phonon-induced enhancement is observed in the $E_B$ range from zero to at least $\delta^c$. After $\Delta C$ recovers from its minimum, positive values, indicating the entanglement enhancement compared with the phonon-free case, are found for binding energies approximately up to 2.5 - 4 times the value of the splitting $\delta^c$.

## PHENOMENOLOGICAL DEPHASING RATE MODEL

A simple standard approximate method used to model pure dephasing is the introduction of phenomenological pure dephasing rates [5, 17]. Instead of the exact treatment of the continuum of longitudinal acoustic phonons, a Lindblad-type operator is introduced. Here, we follow the methodology of Ref. [5] and use the operator

$$\mathcal{L}_{PD}\left[\hat{\rho}\right] = -\frac{1}{2} \sum_{\substack{\chi,\chi' \\ \chi \neq \chi'}} \gamma_{PD} \, |\chi\rangle\langle\chi|\hat{\rho}|\chi'\rangle\langle\chi'|, \tag{S6}$$

with $\chi, \chi' \in \{G, X_H, X_V, B\}$ and a pure dephasing rate $\gamma_{PD}$. Typical values for $\gamma_{PD}$ correspond to several µeV. In Fig. S4, results are shown for the two configurations discussed in Fig. 1 of the main text and Fig. S2, where phonon-induced enhancement of photon entanglement has been found in simulations fully accounting for phonons on a microscopic level.

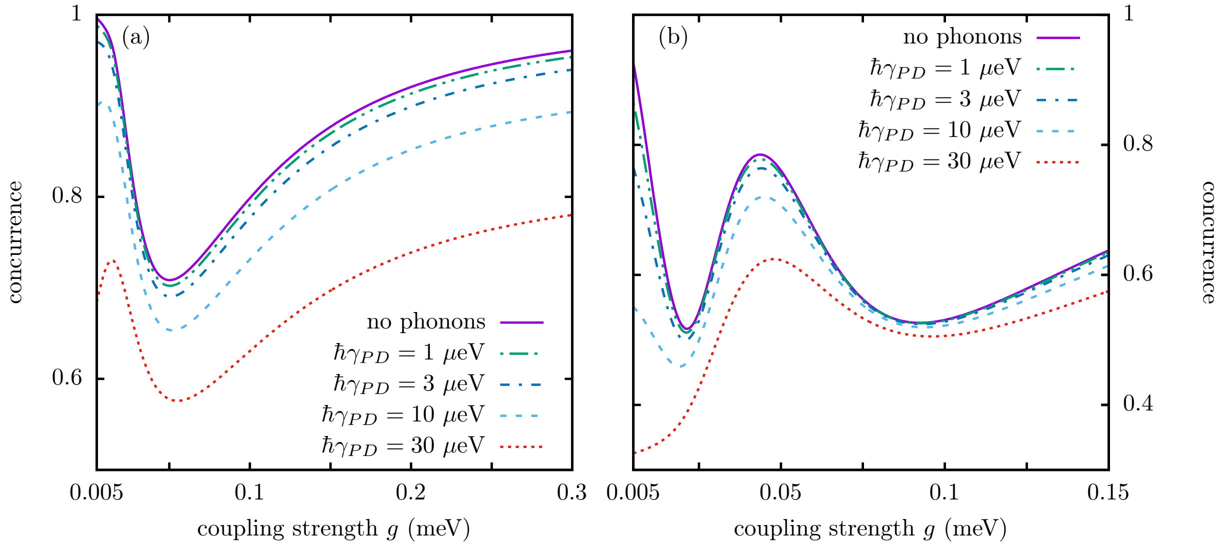


FIG. S4. Results obtained using a phenomenological pure dephasing rate model with different rates $\gamma_{PD}$ instead of the exact path-integral method. (a) Results for the configuration discussed in Fig. 1 in the main text with parameters $\delta = 0.1$ meV, $\kappa = 0.025$ ps$^{-1}$. (b) Results for the configuration discussed in Fig. S2 with parameters $\delta^c = 0.07$ meV, $\kappa = 0.05$ ps$^{-1}$.

Clearly, the effect of phonon-enhanced entanglement does not occur, as the introduction of a pure dephasing rate just leads to a reduction of the concurrence. Furthermore, when one models a higher temperature with a higher loss rate $\gamma_{PD}$, an increasing temperature results always in a decreasing degree of entanglement. Thus, the simple phenomenological rate approximation is not sufficient to model the system dynamics in this situation. This finding further strengthens the explanation of the effect given in the main text where we concluded that the phonon-induced enhancement appears because of a renormalization of the light-matter coupling $g$. This renormalization is, however, absent in the simple rate model and, consequently, the phonon-induced enhancement of photon entanglement does not appear.

## NUMERICAL REMARKS

We use for our simulations a recently developed real-time path-integral algorithm to determine the temporal evolution of the reduced density matrix. Two major achievements enable us to obtain numerically complete results for the dynamics of the biexciton cascade coupled to a continuum of longitudinal acoustic phonons. The first is a translation of concepts originally developed in Hilbert space [18, 19] to Liouville space [20], which allows us to account for non-Hamiltonian contributions, like the Lindblad-type losses, to the dynamics. The second is a reformulation of the algorithm to perform the sum over paths. Instead of the widely used iteration scheme worked out by Makri and Makarov [18, 19] for the so called *augmented density matrix*, only a partially summed augmented density matrix is iterated. A detailed derivation and description of this improved iteration scheme can be found in the supplement of Ref. [21]. For systems like quantum dots coupled to cavities and longitudinal acoustic phonons, the numerical demand is reduced by many orders of magnitude in this way. Two parameters, the step size of the time discretization $\Delta t$ and the number of time steps $N_{\mathrm{mem}}$ used to scan the finite memory, determine the quality of the numerical results. These parameters can be well controlled and we speak of *numerically complete results* when no visible change of the results occurs when further decreasing $\Delta t$ or increasing $N_{\mathrm{mem}}$. For the QD-cavity systems considered in the present paper, numerically converged results are obtained for $\Delta t = 0.5$ ps and $N_{\mathrm{mem}} = 7$.

[1] W. K. Wootters, Quantum Inf. Comput. **1**, 27 (2001).
[2] W. K. Wootters, Phys. Rev. Lett. **80**, 2245 (1998).
[3] M. Cygorek, F. Ungar, T. Seidelmann, A. M. Barth, A. Vagov, V. M. Axt, and T. Kuhn, Phys. Rev. B **98**, 045303 (2018).
[4] G. Pfanner, M. Seliger, and U. Hohenester, Phys. Rev. B **78**, 195410 (2008).

[5] S. Schumacher, J. Förstner, A. Zrenner, M. Florian, C. Gies, P. Gartner, and F. Jahnke, Opt. Express **20**, 5335 (2012).
[6] D. Heinze, A. Zrenner, and S. Schumacher, Phys. Rev. B **95**, 245306 (2017).
[7] M. Cosacchi, M. Cygorek, F. Ungar, A. M. Barth, A. Vagov, and V. M. Axt, Phys. Rev. B **98**, 125302 (2018).
[8] R. M. Stevenson, A. J. Hudson, A. J. Bennett, R. J. Young, C. A. Nicoll, D. A. Ritchie, and A. J. Shields, Phys. Rev. Lett. **101**, 170501 (2008).
[9] S. Bounouar, C. de la Haye, M. Strau, P. Schnauber, A. Thoma, M. Gschrey, J.-H. Schulze, A. Strittmatter, S. Rodt, and S. Reitzenstein, Appl. Phys. Lett. **112**, 153107 (2018).
[10] E. del Valle, New J. Phys. **15**, 025019 (2013).
[11] D. F. V. James, P. G. Kwiat, W. J. Munro, and A. G. White, Phys. Rev. A **64**, 052312 (2001).
[12] A. Vagov, M. Glässl, M. D. Croitoru, V. M. Axt, and T. Kuhn, Phys. Rev. B **90**, 075309 (2014).
[13] M. E. Reimer, M. P. van Kouwen, A. W. Hidma, M. H. M. van Weert, E. P. A. M. Bakkers, L. P. Kouwenhoven, and V. Zwiller, Nano Letters **11**, 645 (2011).
[14] F. Ding, R. Singh, J. D. Plumhof, T. Zander, V. Křápek, Y. H. Chen, M. Benyoucef, V. Zwiller, K. Dörr, G. Bester, A. Rastelli, and O. G. Schmidt, Phys. Rev. Lett. **104**, 067405 (2010).
[15] R. Trotta, P. Atkinson, J. D. Plumhof, E. Zallo, R. O. Rezaev, S. Kumar, S. Baunack, J. R. Schrter, A. Rastelli, and O. G. Schmidt, Advanced Materials **24**, 2668 (2012).
[16] R. Trotta, E. Zallo, E. Magerl, O. G. Schmidt, and A. Rastelli, Phys. Rev. B **88**, 155312 (2013).
[17] F. Troiani, J. I. Perea, and C. Tejedor, Phys. Rev. B **74**, 235310 (2006).
[18] N. Makri and D. E. Makarov, J. Chem. Phys. **102**, 4600 (1995).
[19] N. Makri and D. E. Makarov, J. Chem. Phys. **102**, 4611 (1995).
[20] A. M. Barth, A. Vagov, and V. M. Axt, Phys. Rev. B **94**, 125439 (2016).
[21] M. Cygorek, A. M. Barth, F. Ungar, A. Vagov, and V. M. Axt, Phys. Rev. B **96**, 201201(R) (2017).
